# Supplementary material for: Adaptive Anytime Multi-Agent Path Finding Using Bandit-Based Large Neighborhood Search
Source: arXiv:2312.16767 source file (2024-01-01)
Supplement: Supplementary file 1 [file appendix.tex]

\cleardoublepage
\appendix
\onecolumn
\section{Appendix -- Technical Details, Hyperparameters, and Additional Results}

\subsection{Infrastructure}

\subsubsection{Software and Libraries}

The code for the algorithms (MAPF-LNS, multi-armed bandits, etc.) was developed and run using \texttt{C++ 14} with \texttt{boost 1.81.0} and \texttt{eigen 3.3} as third party libraries. We used \texttt{CMake 3.16.3} to build the code.
The provided \texttt{README.md} explains how to build and run our code to reproduce the results in Section \ref{sec:experiments} in the paper.

\subsubsection{Computing Infrastructure}

All experiments were run on a computing cluster of fifteen x86\_64 GNU/Linux (Ubuntu 18.04.5 LTS) machines with i7 @ 2.4 GHz CPU and 16 GB RAM similarly to \cite{HuangAAAI22}.

\subsection{Hyperparameters}

\subsubsection{Hyperparameter Choice}\label{subsec:appendix_hyperparameters}

All hyperparameters used by the respective BALANCE variants as reported in Section \ref{sec:experiments} are listed in Table \ref{tab:common_hyperparameters}. Most values are based on the default configuration of the public code of \cite{li2022lns2}\footnote{The default hyperparameters can also be found in the code in \texttt{src/driver.cpp}.}. We report the ranges for values that have been tried during our experiments.

For Thompson Sampling, we use an \emph{uninformed prior}, i.e., a prior distribution without exploiting particular knowledge about the underlying setting, where we assume a flat Normal distribution $\mathcal{N}(\mu_0, \sigma_0^2)$ which is close to a random uniform distribution. Therefore, we set the mean $\mu_0 = 0$. The variance $\sigma_0^2 = \frac{1}{\lambda_0 \tau}$ of the Normal distribution needs to be large (ideally infinite) thus we set $\lambda_0 = 0.01$. Since $\tau$ follows a Gamma distribution $\textit{Gamma}(\alpha_{0},\beta_{0})$ with expectation $\mathbb{E}(\tau) = \frac{\alpha_{0}}{\beta_{0}}$, $\alpha_{0}$ and $\beta_{0}$ should be chosen such that $\frac{\alpha_{0}}{\beta_{0}} \rightarrow 0$. Given the hyperparameter space of $\alpha_{0} \geq 1$ and $\beta_{0} \geq 0$, we set $\alpha_{0} = 1$ and $\beta_{0} = 100$.
We directly adopt these prior values in our experiments as proposed in \cite{bai2013bayesian,bai2014thompson} without further tuning.

\begin{table*}[!ht]
\centering
\caption{Hyperparameters and their respective final values used by the respective BALANCE variants evaluated in the paper. We also list the numbers or ranges that have been tried during development of the paper.}
\begin{tabular}{|L{2.25cm}|L{2.25cm}|L{2.25cm}|L{9.1cm}|} \hline
Hyperparameter & Final Value & Numbers/Range & Description\\ \hline\hline
$E$ & $5$ & \{$1$, $2$, $3$, $4$, $5$, $6$, $7$\} & Number of neighborhood options. After $E = 5$, the performance deteriorates in most cases because replanning for neighborhood sizes $N > 64$ requires significant compute therefore limiting the number of LNS iterations.\\\hline
Replanning & PP (prioritized planning) & PP (prioritized planning) & MAPF algorithm for fast replanning of destroyed paths. PP (prioritized planning) from \cite{silver2005cooperative} is the default setting, which was adopted in our experiments. \\\hline
Initial solver & LNS2 with PP & LNS2 with PP & To avoid extensive tuning according to \cite{HuangAAAI22}, we simply use LNS according to \cite{li2022lns2} with a similar BALANCE scheme to the actual procedure of Figure \ref{fig:balance_scheme} and Algorithm \ref{algorithm:BALANCE} in the paper. The initial solver uses the same MAB algorithm as the main LNS2 procedure. \\\hline
$\xi$ & $1,000$ & \{$10$, $100$, $1000$, $10000$\} & Exploration constant for UCB1. There is no significant difference between $1,000$ and $10,000$ but performance gets worse when $\xi < 1,000$ due to insufficient exploration. It is generally recommended to choose a high value of $\xi$ in large-scale scenarios with many agents. \\\hline
$\mu_0$ & $0$ & $0$ & Prior parameter for Thompson Sampling. The value is directly adopted from \cite{bai2013bayesian,bai2014thompson}. \\\hline
$\lambda_0$ & $0.01$ & $0.01$ & Prior parameter for Thompson Sampling. The value is directly adopted from \cite{bai2013bayesian,bai2014thompson}. \\\hline
$\alpha_0$ & $1$ & $1$ & Prior parameter for Thompson Sampling. The value is directly adopted from \cite{bai2013bayesian,bai2014thompson}. \\\hline
$\beta_0$ & $100$ & $100$ & Prior parameter for Thompson Sampling. The value is directly adopted from \cite{bai2013bayesian,bai2014thompson}. \\\hline
\end{tabular}\label{tab:common_hyperparameters}
\end{table*}

\subsubsection{Random Seed}

The random seed can be set by the option \texttt{--seed} when running the code. The default seed according to the public code is zero, which we did not modify in our experiments. We used the 25 random scenarios per map provided by the MAPF benchmark instead to evaluate our approach in diverse instances.

\subsection{Incremental Update of BALANCE Statistics}

For statistics $\Delta$ as explained in Section \ref{subsec:balance_instantiations} for roulette wheel selection, UCB1, and Thompson Sampling, we track the \emph{weight} or \emph{sum of rewards} $w_k = \sum^{T_k}_{c=1} x^{(c)}_{k}$ and the \emph{arm selection count} $T_k$ for each arm $k$. For Thompson Sampling, we additionally track the \emph{sum of squared rewards} $q_k = \sum^{T_k}_{c=1} (x^{(c)}_{k})^2$

After selecting arm $k$ and observing reward $x^{\textit{new}}_{k}$, the values of $w_k$, $T_k$, and $q_k$ are updated incrementally as follows:
\begin{align*}
w_k &\leftarrow w_k + x^{\textit{new}}_{k}\\
T_k &\leftarrow T_k + 1\\
q_k &\leftarrow q_k + (x^{\textit{new}}_{k})^2
\end{align*}

Using the incrementally updatable variables $w_k$, $T_k$, and $q_k$, the MAB selection rules can be implemented as explained in Section \ref{subsec:balance_instantiations}. In the following, we denote the actual implemented form in {\color{blue}\textbf{boldface and blue}} to emphasize its constant computation time.

\subsubsection{Roulette Wheel Selection}
The weights $w_k$ can be used directly to compute the selection probabilities of each arm $k$ as explained in Section \ref{subsec:balance_instantiations}.

\subsubsection{UCB1}
Given the weights $w_k$ and selection counts $T_k$, the average reward $\overline{x}_k$ and the total number of arm selections $K$ are computed as follows:
\begin{align*}
\overline{x}_k &\leftarrow {\color{blue}\mathbf{\frac{1}{T_k}w_k}} = \frac{1}{T_k}\sum^{T_k}_{c=1} x^{(c)}_{k}\\
T &\leftarrow {\color{blue}\mathbf{{\sum^{K}_{k=1}T_k}}}
\end{align*}

\subsubsection{Thompson Sampling}
Given the weights $w_k$ and selection counts $T_k$, the average reward $\overline{x}_k$ is computed identically as for UCB1. In addition, the variance $\sigma^{2}_k$ is computed with $q_k$ and $\overline{x}_k$ as follows:
\begin{align*}
\sigma^{2}_k \leftarrow {\color{blue}\mathbf{{\frac{1}{T_k}q_k - (\overline{x}_k)^2}}} = \frac{1}{T_k}\sum^{T_k}_{c=1} (x^{(c)}_{k})^2 - (\overline{x}_k)^2 = \frac{1}{T_k}\sum_{c = 1}^{T_k} (x^{(c)}_{k} - \overline{x}_k)^2
\end{align*}

\subsection{Additional Results}

Based on the results from the state-of-the-art comparison in Section \ref{subsec:star_results}, we evaluate the performance of \emph{BALANCE (Thompson)}, \emph{BALANCE (UCB1)}, and \emph{BALANCE (Roulette)} with significantly less time budget than the state-of-the-art (which is run with 60 seconds), namely with 15 and 30 seconds of search time. The results are shown in Figure \ref{fig:balance_results_15} and \ref{fig:balance_results_30} respectively. Except for \texttt{den520d}, all BALANCE variants clearly outperform the state-of-the-art with a time budget of just 15 seconds. If the time budget is 30 seconds, then BALANCE is always superior.

\begin{figure*}
	\centering
	\includegraphics[width=0.9\textwidth]{img/balance_results_15.pdf}
     \caption{Sum of delays for different variants of BALANCE compared with state-of-the-art anytime MAPF-LNS and MAPF-ML-LNS for different number of agents $m$. The performance values of MAPF-LNS and MAPF-ML-LNS are taken from \cite{HuangAAAI22}. Our experiments are run on the same hardware specification with a time budget of 15 seconds (\textbf{Note}: MAPF-LNS and MAPF-ML-LNS had a time budget of 60 seconds). Shaded areas show the 95\% confidence interval. The legend at the top applies across all plots.}
     \label{fig:balance_results_15}
\end{figure*}

\begin{figure*}
	\centering
	\includegraphics[width=0.9\textwidth]{img/balance_results_30.pdf}
     \caption{Sum of delays for different variants of BALANCE compared with state-of-the-art anytime MAPF-LNS and MAPF-ML-LNS for different number of agents $m$. The performance values of MAPF-LNS and MAPF-ML-LNS are taken from \cite{HuangAAAI22}. Our experiments are run on the same hardware specification with a time budget of 30 seconds (\textbf{Note}: MAPF-LNS and MAPF-ML-LNS had a time budget of 60 seconds). Shaded areas show the 95\% confidence interval. The legend at the top applies across all plots.}
     \label{fig:balance_results_30}
\end{figure*}
